# Supplementary material for: Spin Hall effects without spin currents in magnetic insulators
Source: arXiv:1803.01294 ancillary file (2019-05-14)
Supplement: Supplementary file 1 [file supp.pdf]

# Supplementary Materials for "Spin Hall effect without spin currents in magnetic insulators"

Hua Chen,[1,2] Qian Niu,[3] and Allan H. MacDonald[3]

[1]*Department of Physics, Colorado State University, Fort Collins, CO 80523, USA*
[2]*School of Advanced Materials Discovery, Colorado State University, Fort Collins, CO 80523, USA*
[3]*Department of Physics, University of Texas at Austin, Austin, TX 78712, USA*

## GAUGE TRANSFORMATION IDENTITIES

In this section we prove several identities used in the main text related to gauge transformations.

We start from the projection operators $P_{\mathbf{k}}$ and $Q_{\mathbf{k}}$ defined in the main text. Under an arbitrary unitary transformation $U_{\mathbf{k}}$ restricted in the occupied space, we have

$$P'_{\mathbf{k}} = \sum_n |u'_{n\mathbf{k}}\rangle\langle u'_{n\mathbf{k}}| = \sum_{nml} |u_{m\mathbf{k}}\rangle U_{mn} U^\dagger_{nl} \langle u_{l\mathbf{k}}| = \sum_m |u_{m\mathbf{k}}\rangle\langle u_{m\mathbf{k}}| = P_{\mathbf{k}}, \tag{1}$$

which means $P_{\mathbf{k}}$ is invariant under the gauge transformation $U_{\mathbf{k}}$. Note $m, n, l$ are all restricted in the occupied space. Apparently $Q_{\mathbf{k}} = 1 - P_{\mathbf{k}}$ is also invariant under $U_{\mathbf{k}}$. Moreover, since $Q_{\mathbf{k}}$ only has nonzero matrix elements in the unoccupied space,

$$Q_{\mathbf{k}} U_{\mathbf{k}} = U_{\mathbf{k}} Q_{\mathbf{k}} = 0. \tag{2}$$

We then show that the (periodic part) of the position operator sandwiched between $P_{\mathbf{k}}$ and $Q_{\mathbf{k}}$ transforms as normal gauge invariant quantities under $U_{\mathbf{k}}$. To this end we start from a representation in which the position operator is $\mathbf{r} = i\partial_{\mathbf{k}}$. Under $U_{\mathbf{k}}$ it acquires an additional term $iU^\dagger_{\mathbf{k}}\partial_{\mathbf{k}}U_{\mathbf{k}}$. However,

$$P_{\mathbf{k}} U^\dagger_{\mathbf{k}} \partial_{\mathbf{k}} U_{\mathbf{k}} Q_{\mathbf{k}} = P_{\mathbf{k}} \partial_{\mathbf{k}} (U^\dagger_{\mathbf{k}} U_{\mathbf{k}}) Q_{\mathbf{k}} - P_{\mathbf{k}} (\partial_{\mathbf{k}} U^\dagger_{\mathbf{k}}) U_{\mathbf{k}} Q_{\mathbf{k}} = 0, \tag{3}$$

where we have used Eq. 2. Similarly

$$Q_{\mathbf{k}} U^\dagger_{\mathbf{k}} \partial_{\mathbf{k}} U_{\mathbf{k}} P_{\mathbf{k}} = 0. \tag{4}$$

Thus under $U_{\mathbf{k}}$ we have

$$P_{\mathbf{k}} \mathbf{r} Q_{\mathbf{k}} \to U^\dagger_{\mathbf{k}} (P_{\mathbf{k}} \mathbf{r} Q_{\mathbf{k}}) U_{\mathbf{k}}, \;\; Q_{\mathbf{k}} \mathbf{r} P_{\mathbf{k}} \to U^\dagger_{\mathbf{k}} (Q_{\mathbf{k}} \mathbf{r} P_{\mathbf{k}}) U_{\mathbf{k}}. \tag{5}$$

Finally we prove the perturbed part of the density matrix $\rho^{(1)}$ transforms as $U^\dagger_{\mathbf{k}}\rho^{(1)}U_{\mathbf{k}}$. This is most easily seen from the equation

$$[H_0, \rho^{(1)}] = -[H_e, \rho^{(0)}]. \tag{6}$$

Since $\rho^{(1)}$ can only have cross-gap matrix elements, and $H_0$ commutes with $P_{\mathbf{k}}$ and $Q_{\mathbf{k}}$, the left hand side of Eq. 6 can be rewritten as

$$[H_0, \rho^{(1)}] = P_{\mathbf{k}} [H_0, \rho^{(1)}] Q_{\mathbf{k}} + Q_{\mathbf{k}} [H_0, \rho^{(1)}] P_{\mathbf{k}}. \tag{7}$$

One can then multiply both sides of Eq. 6 by $P_{\mathbf{k}}$ (from left), $Q_{\mathbf{k}}$ (from right) or $Q_{\mathbf{k}}$ (from left), $P_{\mathbf{k}}$ (from right). Either way, $H_e$ which is proportional to $\mathbf{r}$ is always sandwiched between $P_{\mathbf{k}}$ and $Q_{\mathbf{k}}$. Thus under $U_{\mathbf{k}}$ the right hand side of Eq. 6 transforms as an ordinary gauge-invariant operator: $\hat{O} \to U^\dagger_{\mathbf{k}}\hat{O}U_{\mathbf{k}}$. Since $H_0$ also transforms as $H_0 \to U^\dagger_{\mathbf{k}} H_0 U_{\mathbf{k}}$, we can finally multiply both sides by $U_{\mathbf{k}}$ (from left) and $U^\dagger_{\mathbf{k}}$ (from right), and arrive at the same equation as Eq. 6 by identifying

$$U_{\mathbf{k}} \rho^{(1)\prime} U^\dagger_{\mathbf{k}} = \rho^{(1)}, \text{ or } \rho^{(1)\prime} = U^\dagger_{\mathbf{k}} \rho^{(1)} U_{\mathbf{k}}. \tag{8}$$

## GROUND STATE SPIN DENSITY POLARIZATION OF A G-TYPE ANTIFERROMAGNET

In this section we calculate the ground state spin density polarization of a G-type antiferromagnet on a simple cubic lattice. G-type means that any magnetic moment is antiparallel with all of of its nearest neighbors. A cubic G-type antiferromagnetic ordering can exist in e.g., perovskite materials. A simple cubic lattice is bipartite and can be viewed as a fcc lattice with two sublattices, on which the two staggered magnetic moments are sitting respectively. The positions of the magnetic moments and the unit cell parameters are

$$\begin{aligned} &A:\,(0,0,0),\;\; B:\,a(1,0,0), \\ &\mathbf{a}_1=a(0,1,1),\;\; \mathbf{a}_2=a(1,0,1),\;\; \mathbf{a}_3=a(1,1,0), \\ &\mathbf{b}_1=(-\pi,\pi,\pi)/a,\;\; \mathbf{b}_2=(\pi,-\pi,\pi)/a,\;\; \mathbf{b}_3=(\pi,\pi,-\pi)/a, \end{aligned} \tag{9}$$

where $\mathbf{a}_i$ and $\mathbf{b}_i$ are the lattice vectors in the direct and the reciprocal spaces, respectively, and $a$ is the nearest neighbor distance.

The Hamiltonian for an $s$-electron hopping between nearest neighbors with staggered exchange fields due to the antiferromagnetic order on this lattice is

$$H=-\sum_{\langle im,jn\rangle\alpha} t c^\dagger_{im\alpha}c_{jn\alpha}-\sum_{im\alpha\beta}(-1)^m\Delta c^\dagger_{im\alpha}\sigma^z_{\alpha\beta}c_{im\beta}+h.c. \tag{10}$$

where $i,j$ label magnetic unit cell, $m,n$ label sublattices, $\alpha,\beta$ label spin, and $\Delta$ is the size of the staggered exchange field along $z$.

It is important to note that in writing down the staggered Zeeman term we have made the implicit choice that $\langle\mathbf{r}|c^\dagger_{iB\alpha}|0\rangle$ is localized on site B in the $i$th unit cell. In other words, we have chosen a gauge that shifts the Wannier functions for the B sublattices away from the unit cell origin. After the Fourier transform

$$c^\dagger_{im\alpha}=\frac{1}{N}\sum_{\mathbf{k}}e^{-i\mathbf{k}\cdot\mathbf{R}_i}c^\dagger_{\mathbf{k}m\alpha}, \tag{11}$$

the basis function of $c^\dagger_{\mathbf{k}B\alpha}|0\rangle$ has a momentum dependent phase factor $e^{-i\mathbf{k}\cdot\mathbf{r}_B}=e^{-ik_xa}$. Note that we did not include the phase factor in the Fourier transform, which is the way usually done for multi-sublattice tight-binding models. One can also follow this alternate approach, but should keep in mind that doing so means we have performed a gauge transformation, which not only makes the basis function $\mathbf{k}$ independent, but also changes the Berry connection by adding a term of $iU^\dagger\nabla_{\mathbf{k}}U$, which is basically $\mathrm{diag}(\mathbf{r}_A,\mathbf{r}_B)\otimes \mathrm{I}_{2\times 2}$. The momentum space Hamiltonian is

$$H(\mathbf{k})=C^\dagger_{\mathbf{k}}\begin{pmatrix}\Delta\sigma^z & \gamma_{\mathbf{k}}I\\ \gamma^\dagger_{\mathbf{k}}I & -\Delta\sigma^z\end{pmatrix}C_{\mathbf{k}}, \tag{12}$$

where $C_{\mathbf{k}}=(c_{\mathbf{k}A\uparrow},c_{\mathbf{k}A\downarrow},c_{\mathbf{k}B\uparrow},c_{\mathbf{k}B\downarrow})^T$, and

$$\gamma_{\mathbf{k}}=-2t(\cos k_x+\cos k_y+\cos k_z)e^{-ik_xa}. \tag{13}$$

The Hamiltonian can be written into a block diagonal form with the following diagonal blocks

$$H_\uparrow(\mathbf{k})=C^\dagger_{\mathbf{k}\uparrow}\begin{pmatrix}\Delta & \gamma_{\mathbf{k}}\\ \gamma^\dagger_{\mathbf{k}} & -\Delta\end{pmatrix}C_{\mathbf{k}\uparrow},\;\; H_\downarrow(\mathbf{k})=C^\dagger_{\mathbf{k}\downarrow}\begin{pmatrix}-\Delta & \gamma_{\mathbf{k}}\\ \gamma^\dagger_{\mathbf{k}} & \Delta\end{pmatrix}C_{\mathbf{k}\downarrow} \tag{14}$$

The eigenenergies of the two blocks are the same, $E_{\mathbf{k}}=\pm\sqrt{\gamma^2_{\mathbf{k}}+\Delta^2}$. The eigenfunctions of the occupied ($E_{\mathbf{k}}<0$) bands are

$$\begin{aligned} |u_{\uparrow\mathbf{k}}\rangle &= N_{\mathbf{k}}\left(-\frac{\gamma_{\mathbf{k}}}{\sqrt{|\gamma_{\mathbf{k}}|^2+\Delta^2}+\Delta},1\right)^T, \\ |u_{\downarrow\mathbf{k}}\rangle &= N_{\mathbf{k}}\left(1,-\frac{\gamma^\dagger_{\mathbf{k}}}{\sqrt{|\gamma_{\mathbf{k}}|^2+\Delta^2}+\Delta}\right)^T, \\ N_{\mathbf{k}} &= \sqrt{\frac{1}{2}\left(1+\frac{\Delta}{\sqrt{|\gamma_{\mathbf{k}}|^2+\Delta^2}}\right)}. \end{aligned} \tag{15}$$

This set of eigenfunctions of the occupied space are smooth through the Brillouin zone, since $\gamma_{\mathbf{k}}$ is invariant under $\mathbf{k} \to \mathbf{k} + \mathbf{b}_i$. The ground state spin density polarization can thus be calculated from Eq. 3 in the main text:

$$\langle \overleftrightarrow{p}_s \rangle = -\mathrm{Im} \sum_{\mathbf{k}} \left( \langle u_{\uparrow\mathbf{k}} | \mathbf{s} | \nabla_{\mathbf{k}} u_{\uparrow\mathbf{k}} \rangle + \langle u_{\downarrow\mathbf{k}} | \mathbf{s} | \nabla_{\mathbf{k}} u_{\downarrow\mathbf{k}} \rangle \right). \tag{16}$$

It is straightforward to show that the summands are nonzero only for the $z$ component of $\mathbf{s}$, since all the eigenstates are also $\sigma^z$ eigenstates. Moreover, only when the derivative is taken over the phase factor $e^{-ik_x a}$ in the eigenfunctions one can get a contribution. Thus only the $x$ component of the gradient needs to be considered. Finally, one should keep in mind that there is an additional contribution from the momentum dependence of the basis function $|B\alpha\rangle$. One can show that the 2nd term vanishes and the final result is

$$\langle p_s \rangle_{zx} = \sum_{\mathbf{k}} \frac{\hbar}{2} = \frac{\hbar a}{2V_m}, \tag{17}$$

where $V_m = 2a^3$ is the volume of the magnetic unit cell.

## $\delta\langle p_s \rangle_{gi}$ IN THE CONTINUUM KANE-MELE MODEL WITH AN IN-PLANE ZEEMAN FIELD

In this section we give some analytic results of $\delta\langle p_s \rangle_{gi}$ in the continuum version of the Kane-Mele model with an in-plane Zeeman field. The Hamiltonian is

$$H = \hbar v_F (\tau_z \sigma_x k_x + \sigma_y k_y) + \lambda_{so} \tau_z \sigma_z s_z + J s_x \tag{18}$$

The Hamiltonian has a symmetry operator $C \equiv \sigma_z s_y$:

$$C^\dagger H(\mathbf{k}) C = -H(\mathbf{k}),\ \{H(\mathbf{k}), C\} = 0 \tag{19}$$

which makes the energy spectrum particle-hole symmetric. This property allows us to solve the eigenstates by squaring it:

$$H^2 = \epsilon_k^2 + J^2 + \lambda_{so}^2 + 2\epsilon_k J (\cos\phi_k \sigma_x s_x + \sin\phi_k \sigma_y s_x), \tag{20}$$

where $\epsilon_k = \hbar v_F k$, and $\phi_k = \arctan(k_y/k_x)$. Note that $\sigma_x s_x$ and $\sigma_y s_x$ are Dirac $\Gamma$ matrices satisfying

$$\Gamma_i^2 = 1,\ \{\Gamma_i, \Gamma_j\} = 2\delta_{ij}. \tag{21}$$

Therefore the eigenvalues of $H^2$ can be obtained trivially by squaring it again:

$$E^2 = \epsilon_k^2 + J^2 + \lambda_{so}^2 \pm 2\epsilon_k J, \tag{22}$$

which leads to the eigenvalues of $H$:

$$E = \pm\sqrt{(\epsilon_k \pm J)^2 + \lambda_{so}^2}. \tag{23}$$

For convenience we label the four eigenvalues as follows:

$$\begin{aligned} E_1 &= \sqrt{(\epsilon_k + J)^2 + \lambda_{so}^2}, \\ E_2 &= \sqrt{(\epsilon_k - J)^2 + \lambda_{so}^2}, \\ E_3 &= -\sqrt{(\epsilon_k - J)^2 + \lambda_{so}^2} = -E_2, \\ E_4 &= -\sqrt{(\epsilon_k + J)^2 + \lambda_{so}^2} = -E_1. \end{aligned} \tag{24}$$

To get an analytic form of the eigenfunctions, we use two sets of projection operators. One set of projection operators project an arbitrary state in the Hilbert space of $H$ into either of the two degenerate subspaces of $H^2$. In general, for a Hamiltonian consisting of only Dirac $\Gamma$ matrices

$$H = \sum_i g_i \Gamma_i, \tag{25}$$

its eigenstates are particle-hole symmetric, and all particle states as well as all hole states are degenerate. Therefore any state $\psi_+$ in the particle subspace satisfies

$$H\psi_+ = \sum_i g_i \Gamma_i \psi_+ = +\sqrt{\sum_i |g_i|^2}\psi_+ \equiv \rho\psi_+ \tag{26}$$

which leads to

$$\sum_i \frac{g_i}{\rho}\Gamma_i \psi_+ = \psi_+. \tag{27}$$

Similarly, for any hole state $\psi_-$

$$\sum_i \frac{g_i}{\rho}\Gamma_i \psi_- = -\psi_-. \tag{28}$$

We can thus construct two projection operators $P_+$ and $P_-$:

$$P_\pm = \frac{1}{2}\left(1 \pm \sum_i \frac{g_i}{\rho}\Gamma_i\right), \tag{29}$$

which satisfy

$$\begin{aligned} &P_\pm \psi_\pm = \psi_\pm,\ P_\pm \psi_\mp = 0, \\ &P_\pm^2 = P_\pm,\ P_+ P_- = 0,\ P_+ + P_- = 1. \end{aligned} \tag{30}$$

For the Dirac Hamiltonian $H^2$, the projection operators are

$$P_\pm = -\frac{1}{2}(\cos\phi_k \sigma_x s_x + \sin\phi_k \sigma_y s_x \pm 1). \tag{31}$$

By applying, say $P_+$, to an arbitrary state, we will obtain a linear superposition of the two eigenstates belonging to $E_1$ and $E_4 = -E_1$. To get the coefficient for each of them we need to construct another pair of projection operators defined only in this 2-level subspace:

$$\begin{aligned} P_{+1} &= \frac{1}{2}\left(1 + \frac{H}{E_1}\right), \\ P_{+4} &= \frac{1}{2}\left(1 - \frac{H}{E_1}\right), \end{aligned} \tag{32}$$

which have similar properties as Eq. 30. Similarly the projection operators for the two eigenstates belonging to $E_2$ and $E_3$ are

$$\begin{aligned} P_{-2} &= \frac{1}{2}\left(1 + \frac{H}{E_2}\right), \\ P_{-3} &= \frac{1}{2}\left(1 - \frac{H}{E_2}\right). \end{aligned} \tag{33}$$

By starting from an arbitrary state $\psi$, we can obtain the four eigenstates as follows:

$$\begin{aligned} \psi_1 &= N_1 P_{+1} P_+ \psi, \\ \psi_2 &= N_2 P_{-2} P_- \psi, \\ \psi_3 &= N_3 P_{-3} P_- \psi, \\ \psi_4 &= N_4 P_{+4} P_+ \psi, \end{aligned} \tag{34}$$

where $N_1 - N_4$ are normalization factors. We finally arrive at the following expressions for $\psi_1 - \psi_4$:

$$\begin{aligned} \psi_1 &= N_1 \left[(\lambda_{so} + E_1),\, (\epsilon_k + J),\, (\epsilon_k + J)e^{i\phi_k},\, (\lambda_{so} + E_1)e^{i\phi_k}\right]^T \\ \psi_2 &= N_2 \left[-(\lambda_{so} + E_2),\, (\epsilon_k - J),\, -(\epsilon_k - J)e^{i\phi_k},\, (\lambda_{so} + E_2)e^{i\phi_k}\right]^T \\ \psi_3 &= N_3 \left[(\lambda_{so} - E_2),\, -(\epsilon_k - J),\, (\epsilon_k - J)e^{i\phi_k},\, -(\lambda_{so} - E_2)e^{i\phi_k}\right]^T \\ \psi_4 &= N_4 \left[-(\lambda_{so} - E_1),\, -(\epsilon_k + J),\, -(\epsilon_k + J)e^{i\phi_k},\, -(\lambda_{so} - E_1)e^{i\phi_k}\right]^T \end{aligned} \tag{35}$$

with the normalization factors

$$N_1 = \left[2(\lambda_{so}+E_1)^2+2(\epsilon_k+J)^2\right]^{-\frac{1}{2}} \tag{36}$$
$$N_2 = \left[2(\lambda_{so}+E_2)^2+2(\epsilon_k-J)^2\right]^{-\frac{1}{2}}$$
$$N_3 = \left[2(\lambda_{so}-E_2)^2+2(\epsilon_k-J)^2\right]^{-\frac{1}{2}}$$
$$N_4 = \left[2(\lambda_{so}-E_1)^2+2(\epsilon_k+J)^2\right]^{-\frac{1}{2}}$$

Above results are for the valley with $\tau_z = 1$. To get the corresponding expressions for the other valley one needs to do the following substitutions:

$$\epsilon_k \to -\epsilon_k,\ \phi_k \to -\phi_k,\ \lambda_{so} \to -\lambda_{so}. \tag{37}$$

Having both the eigenenergies and the eigenfunctions, we can calculate $\delta\langle\overleftrightarrow{p}_s\rangle_{gi}$. Note that strictly speaking the projection operators $P_\pm$ are ill-defined at $k = 0$, but it should not influence the gauge-invariant part of $\delta\langle\overleftrightarrow{p}_s\rangle$. Using Eq. 10 in the main text one can write $\delta\langle\overleftrightarrow{p}_s\rangle_{gi}$ as

$$\delta\langle\overleftrightarrow{p}_s\rangle_{gi} = -e\hbar^2\mathbf{E}\cdot\int\frac{d^2k}{(2\pi)^2}\sum_{n\in o}\sum_{m\in u}\left[\sum_{l\in u}\frac{\mathrm{Re}(\mathbf{v}_{nm}\mathbf{s}_{ml}\mathbf{v}_{ln})}{(E_{m\mathbf{k}}-E_{n\mathbf{k}})^2(E_{n\mathbf{k}}-E_{l\mathbf{k}})}-\sum_{l\in o}\frac{\mathrm{Re}(\mathbf{v}_{mn}\mathbf{s}_{nl}\mathbf{v}_{lm})}{(E_{m\mathbf{k}}-E_{n\mathbf{k}})^2(E_{m\mathbf{k}}-E_{l\mathbf{k}})}\right]. \tag{38}$$

The velocity operators for the current model are

$$\mathbf{v} = \frac{\partial H}{\hbar\partial\mathbf{k}} = v_F\tau_z\sigma_x\hat{x}+v_F\sigma_y\hat{y}. \tag{39}$$

Substituting the eigenfunctions $\psi_i$ (Eqs. 35 and 36) and the eigenvalues $E_i$ (Eq. 24) together with the expressions of the velocity operators Eq. 39 and the spin operators into Eq. 38, we can in principle get the analytic results of $\delta\langle\overleftrightarrow{p}_s\rangle_{gi}$. However, different from the Berry curvature of a gapped Dirac cone which is independent of $\phi_k$, the integrand in Eq. 38 is $\phi_k$ dependent, making it difficult to calculate the integral. We thus resort to Mathematica and expand the result to the 1st order in $J$, i.e., by treating the in-plane Zeeman field as a perturbation. The results are (including contributions from both valleys)

$$\delta\langle p_s\rangle_{gi}(x,y,y) = -\frac{e\hbar JE}{60\pi v_F^2\lambda_{so}^2}+O(J^2), \tag{40}$$
$$\delta\langle p_s\rangle_{gi}(x,x,y) = \delta\langle p_s\rangle_{gi}(x,z,y) = 0,$$
$$\delta\langle p_s\rangle_{gi}(y,y,x) = \frac{e\hbar JE}{60\pi v_F^2\lambda_{so}^2}+O(J^2),$$
$$\delta\langle p_s\rangle_{gi}(y,x,x) = \delta\langle p_s\rangle_{gi}(y,z,x) = 0,$$

where the three indices in the parentheses label the directions of the electric field, the spin in $p_s$, and the spatial direction in $p_s$. These results mean that when the Zeeman field is along the same direction as the electric field, set as $\hat{x}$, there should be spin accumulation along the edges perpendicular to $y$, and the direction of the accumulated spin is also along $y$, pointing to the outside of the edge. In contrast, when the electric field (along $y$) is perpendicular to the Zeeman field (along $x$), the spin accumulation will be along the edges perpendicular to $x$ with the same magnitude and pointing to the outside of the edge. The size of the spin density polarization is proportional to the Zeeman field and inversely proportional to the Fermi velocity and the spin-orbit coupling (i.e., the gap) squared, as is typically expected for an inter-band response. Thus when the spin-orbit coupling gap is much larger than the Zeeman field the effect will be tiny. We have compared Eq. 40 with numerical results using the corresponding tight-binding Hamiltonian for an extended system and found they agree very well when $J \ll \lambda_{so}$, but the results can be several times smaller than that calculated for a relatively narrow ribbon in the main text. The reason is that there are also edge contributions to $\delta\langle p_s\rangle_{gi}$, which will however vanish as the width of the ribbon goes to infinity (Fig. 3 in main text).
